# Supplementary material for: Sharing Equality is Linear
Source: arXiv:1907.06101 source file (2019-07-13)
Supplement: Supplementary file 1 [file algorithm-visited.tex]

% !TEX root = main.tex

\clearpage
\section{Blind check with \texttt{visiting} and no queue}

\begin{algorithm}
 \SetArgSty{textrm}
 \SetNlSty{}{}{} 
 \DontPrintSemicolon

 % Header
 \KwData{an initial state}
 \KwResult{either \FAIL or a final state}
 \BlankLine

 % Blind Sharing Check
 \procedure{\BlindSharingCheck{}}{
 \For{\textbf{every} node $\node$}
  {\lIf{$\pointer{\node}$ undefined}{\label{alg:no-queue-main-while}$\SetCanonic{\node, \node}$}}
 }
 
 \BlankLine
 
 % SetCanonic
 \procedure{$\SetCanonic{\node, \cannode}$}{
    \lIf{$\labelop\node \neq \labelop\cannode$}{\FAIL{}}
    $\visiting\node \defeq \true$\; 
    $\pointer \node \defeq \cannode$\;
    
    \For{\textbf{every} parent $\nodetwo$ of $\node$}{%
      \lIf{$\visiting\nodetwo$}{\FAIL{}} 
      \lIf{$\pointer{\nodetwo}$ undefined}{$\SetCanonic{\nodetwo,\nodetwo}$}
    }
    
    \If{$\node$ and $\cannode$ have children resp. $\node_1,\node_2$ and $\nodetwo_1,\nodetwo_2$}{
      create undirected query edges $\node_1 \sim \nodetwo_1$ and $\node_2 \sim \nodetwo_2$\;
    }

    \For{\textbf{every} $\sim$-sibling $\nodetwo$ of $\node$}{ 
      \lIf{$\pointer{\nodetwo}$ undefined}{$\SetCanonic{\nodetwo,\cannode}$}
      \lElseIf{$\pointer\nodetwo \neq \cannode$}{\FAIL{}}
    }
    
    $\visiting\node \defeq \false$
 }
 
 \caption{Blind sharing check}
 \label{alg:no-queue-sharing-check}
\end{algorithm}
