# Supplementary material for: Sharing Equality is Linear
Source: arXiv:1907.06101 source file (2019-07-13)
Supplement: Supplementary file 2 [file old_algorithm.tex]

% !TEX root = main.tex
\begin{algorithm}
 \SetArgSty{textrm}
 \SetAlgoLined
 % \DontPrintSemicolon

 \KwData{an initial state}
 \KwResult{either \FAIL or a final state}
 \BlankLine

 \SetKwProg{myfinish}{Procedure}{}{}
 \SetKwProg{mypush}{Procedure}{}{}
 \SetKwProg{mypropagate}{Procedure}{}{}
 \SetKwProg{mymain}{Procedure}{}{}

 \SetKw{and}{and}
 \SetKw{nott}{not}

 % Blind Sharing Check
 \mymain{\main{}}{
 % \tcp{build sharing equivalence}
 \nl \lWhile{there is any alive node $\node$}{\fin{$\node$}\label{alg_start}}
 }
 \BlankLine
 
 % Kill
 \myfinish{\fin{$\wcan$}}{
 $\stack \defeq \emptyset$\label{alg_create}\;
 \leIf{$\pointer \wcan$ is $\cundefined$\label{alg_if_undefi}}{%
 $\pointer \wcan \leftarrow \wcan$\label{alg_assign_canoni}%
 }{%
 \FAIL \label{alg_push_faili}%
 } \nl%
 \lWhile{$\wcan$ has some alive parent $\node$}
 {\label{alg6i}$\fin{\node}$}

 \nl \While{there is an undirected query edge $(\wcan,\node)$\label{alg_while3i}}{%
 \push{$\stack$, $\wcan$, $\node$}\label{alg7i}\;
 delete undirected query edge $(\wcan,\node)$\;
 }

 \While{\nott $\stack$.empty()\label{alg_while1}}{
 $\sthead\defeq \stack$.head()\; \label{alg_pop}
 \nl \lWhile{$\sthead$ has some alive parent $\node$}{$\fin{\node}$\label{alg6}}
 \nl \While{there is an undirected query edge $(\sthead,\node)$\label{alg_while3}}{
 \push{$\stack$, $\wcan$, $\node$}\label{alg7}\;
 delete undirected query edge $(\sthead,\node)$\label{alg8}\;
 }
 \nl $\stack$.pop()\label{alg11}\label{alg_end_while1}\;
 mark $\sthead$ dead\;
 }
 \nl mark $\wcan$ dead\label{alg12}\;
 }

 \BlankLine
 \mypush{\push{$\stack$, $\wcan$, $\node$}}{
 \uIf{$\pointer \node$ is $\cundefined$\label{alg_if_undef}}{
 \nl       $\pointer \node \defeq \wcan$\label{alg_assign_canon}\;
 \nl       $\stack$.push($\node$)\label{alg_push}\;
 \nl \lIf{$\wcan$, $\node$ have different labels}{\FAIL\label{alg_clash}}
 \If{$\wcan$ and $\node$ have children resp. $\wcan_1,\wcan_2$ and $\node_1,\node_2$}{
 \nl       create undirected query edges $(\wcan_1, \node_1)$ and $(\wcan_2, \node_2)$\label{alg_prop_app}\;}
 }
 \nl \lElseIf{$\pointer \node \neq \wcan$}{\FAIL\label{alg_push_fail}}
 }

 \caption{\Core sharing check}
 \label{alg:sharing-check}
\end{algorithm}
